# Supplementary material for: Galaxy Zoo Builder: Morphological Dependence of Spiral Galaxy Pitch Angle
Source: arXiv:2105.04500 source file (2021-05-10)
Supplement: Supplementary file 1 [file appendix.tex]

% !TEX root = ../main.tex
